# Supplementary material for: Focused Adaptation of Dynamics Models for Deformable Object Manipulation
Source: arXiv:2209.14261 source file (2023-03-15)
Supplement: Supplementary file 1 [file supp.tex]

\section{Supplemental Materials}

\subsection{The behavior of FOCUS on Plant Watering}

Add a figure showing how FOCUS quickly focuses on pours that do not interact with the plant, improving data efficiency

Explain how/why the water experiment can fail if number of trails per iteration are low and no good pours are obtained.

\subsection{The weighting fuction}

Expand upon how the weighting function / hyperparameters influence things

\subsection{Additional Real Robot Results for Rope Manipulation}

Here we repeat the real-world rope manipulation adaptation experiment, but we now use a different starting configuration than the one used in Section \ref{sec:real_rope_experiments}. Previously, the start state used was the same as the one used for training. This could give an advantage to the AllDataNoMDE baseline, since it was trained on all data collected from around this starting state. If we vary the starting state, our hypothesis is that the AllDataNoMDE baseline will be out of distribution and will not generalize well, whereas FOCUS will not be out of distribution and will generalize. This is because the free-space dynamics are consistent across the different free-space start states, whereas the dynamics of contact which may have been memorized by the AllDataNoMDE baseline are not as easily generalized.
